# Supplementary material for: Beyond Training: How Workers Discover Value in Enterprise AI
Source: arXiv:2502.13281 source file (2025-10-06)
Supplement: Supplementary file 1 [file 8_Appendix.tex]

\appendix
\section{Interview Guidelines}

\subsection*{Phase 1: Learnability \& Onboarding}
\begin{enumerate}
    \item Did you have specific onboarding or training to learn how to use Copilot?
    \item Through which mediums have you learned to use Copilot most? (e.g., trainings in your workplace, workshops, online videos, social media, your own explorations, trial and error, etc.)
    \begin{enumerate}[label*=\arabic*.]
        \item Was it through any of these mediums?
    \end{enumerate}
    \item Have you had experience using other AI tools either at work or outside of your workplace (e.g., Chat-GPT, Gemini, Claude, etc.)?
    \begin{enumerate}[label*=\arabic*.]
        \item If yes, how long have you been using these tools? What have you used them for?
        \item How have your experiences with these other AI tools helped you understand how Copilot works (e.g., what it does, how it works, its limitations)?
    \end{enumerate}
    \item On a scale of 1 to 10, with 1 being not at all and 10 being completely, how confident do you feel that you truly maximize the capabilities and features offered by Copilot when you work?
    \item Do you and your colleagues at work ever share new information about how to use Copilot (e.g., best practices, new features, discovered limitations)?
    \item What has motivated you to incorporate Copilot into your work practice? (e.g., genuine curiosity, leadership expectations, efficiency improvements)
\end{enumerate}

\subsection*{Phase 2: Last Memorable Bad Time Using Copilot}
\begin{enumerate}
    \item Can you recall a time when you were excited to use Copilot at work to help you accomplish something, but it fell short of your expectations?
    \item In general, what would you say are the biggest limitations of Copilot that you have personally experienced so far?
\end{enumerate}

\subsection*{Phase 3: Last Memorable Good Time Using Copilot}
\begin{enumerate}
    \item Can you recall a time when you were excited to use Copilot at work and it met or exceeded your expectations?
    \item In general, what would you say are the greatest strengths of Copilot that you have personally experienced so far?
\end{enumerate}

\subsection*{Phase 4: General Use of Copilot}
\begin{enumerate}
    \item What are your most common use-cases for Copilot at work?
    \item On a scale of 1 to 10 (1 = not at all, 10 = extremely well), how well does Copilot help you accomplish your tasks on average?
    \item On a scale of 1 to 10 (1 = worse off, 5 = neutral, 10 = extremely beneficial), how has Copilot affected your efficiency at work?
\end{enumerate}
